# Supplementary material for: Decentralized Stream Runtime Verification for Timed Asynchronous Networks
Source: arXiv:2302.00506 source file (2023-02-03)
Supplement: Supplementary file 1 [file appendix.tex]

\section{More Examples}
\label{sec:app:examples}
%For Timed Asynchronous
Unrolling example, plots: arrows of when instant streams are resolved and the prediction of the eqs,...
\begin{example}
  {\footnotesize\begin{lstlisting}[language=LOLA]
    @1{input int a}
    @2{define int b = a[-1|0]
      output int c = b + a}
  \end{lstlisting}}
  We can obtain the $MTR(\InstVar{c}{1})$ as follows:
  \begin{align*}
    &MTR(\InstVar{c}{1}) = \max(\MTRrem(\InstVar{c}{1}),\MTR(\InstVar{b}{1})) = \\
    %remotes
    &= \max(\max(1,\ArrivalTime{a}{c}(\MTR(\InstVar{a}{1}))),\max(\MTRrem(\InstVar{b}{1}))) = \\
    &= \max(\max(1,\ArrivalTime{a}{c}(\MTRrem(\InstVar{a}{1}))),\\
    &       \max(\ArrivalTime{a}{b}(\MTR(\InstVar{a}{1-1})))) = \\
    &= \max(\max(1,\ArrivalTime{a}{c}(1)),\ArrivalTime{a}{b}(\MTRrem(\InstVar{a}{0}))) = \\
    &= \max(\max(1,\ArrivalTime{a}{c}(1)),\ArrivalTime{a}{b}(0)) = \\
    &= \max(\ArrivalTime{a}{c}(1),\ArrivalTime{a}{b}(0)) = \\
  \end{align*}
\end{example}

\AlgorithmProceduresLazy

\begin{example}
  \label{ex:msgs}
  In this example we explain how the message sending happens with the
  topology of the network connecting monitors.
  As we can see in Fig.~\ref{fig:RE_msgs}, a message takes 1 cycle to
  reach the next hop in the path from source to destination.
  Therefore the distance between source and destination will be the
  time that a message needs to arrive from source to destination.
\qed
  \begin{figure}
    \centering
  \includegraphics[scale=0.60]{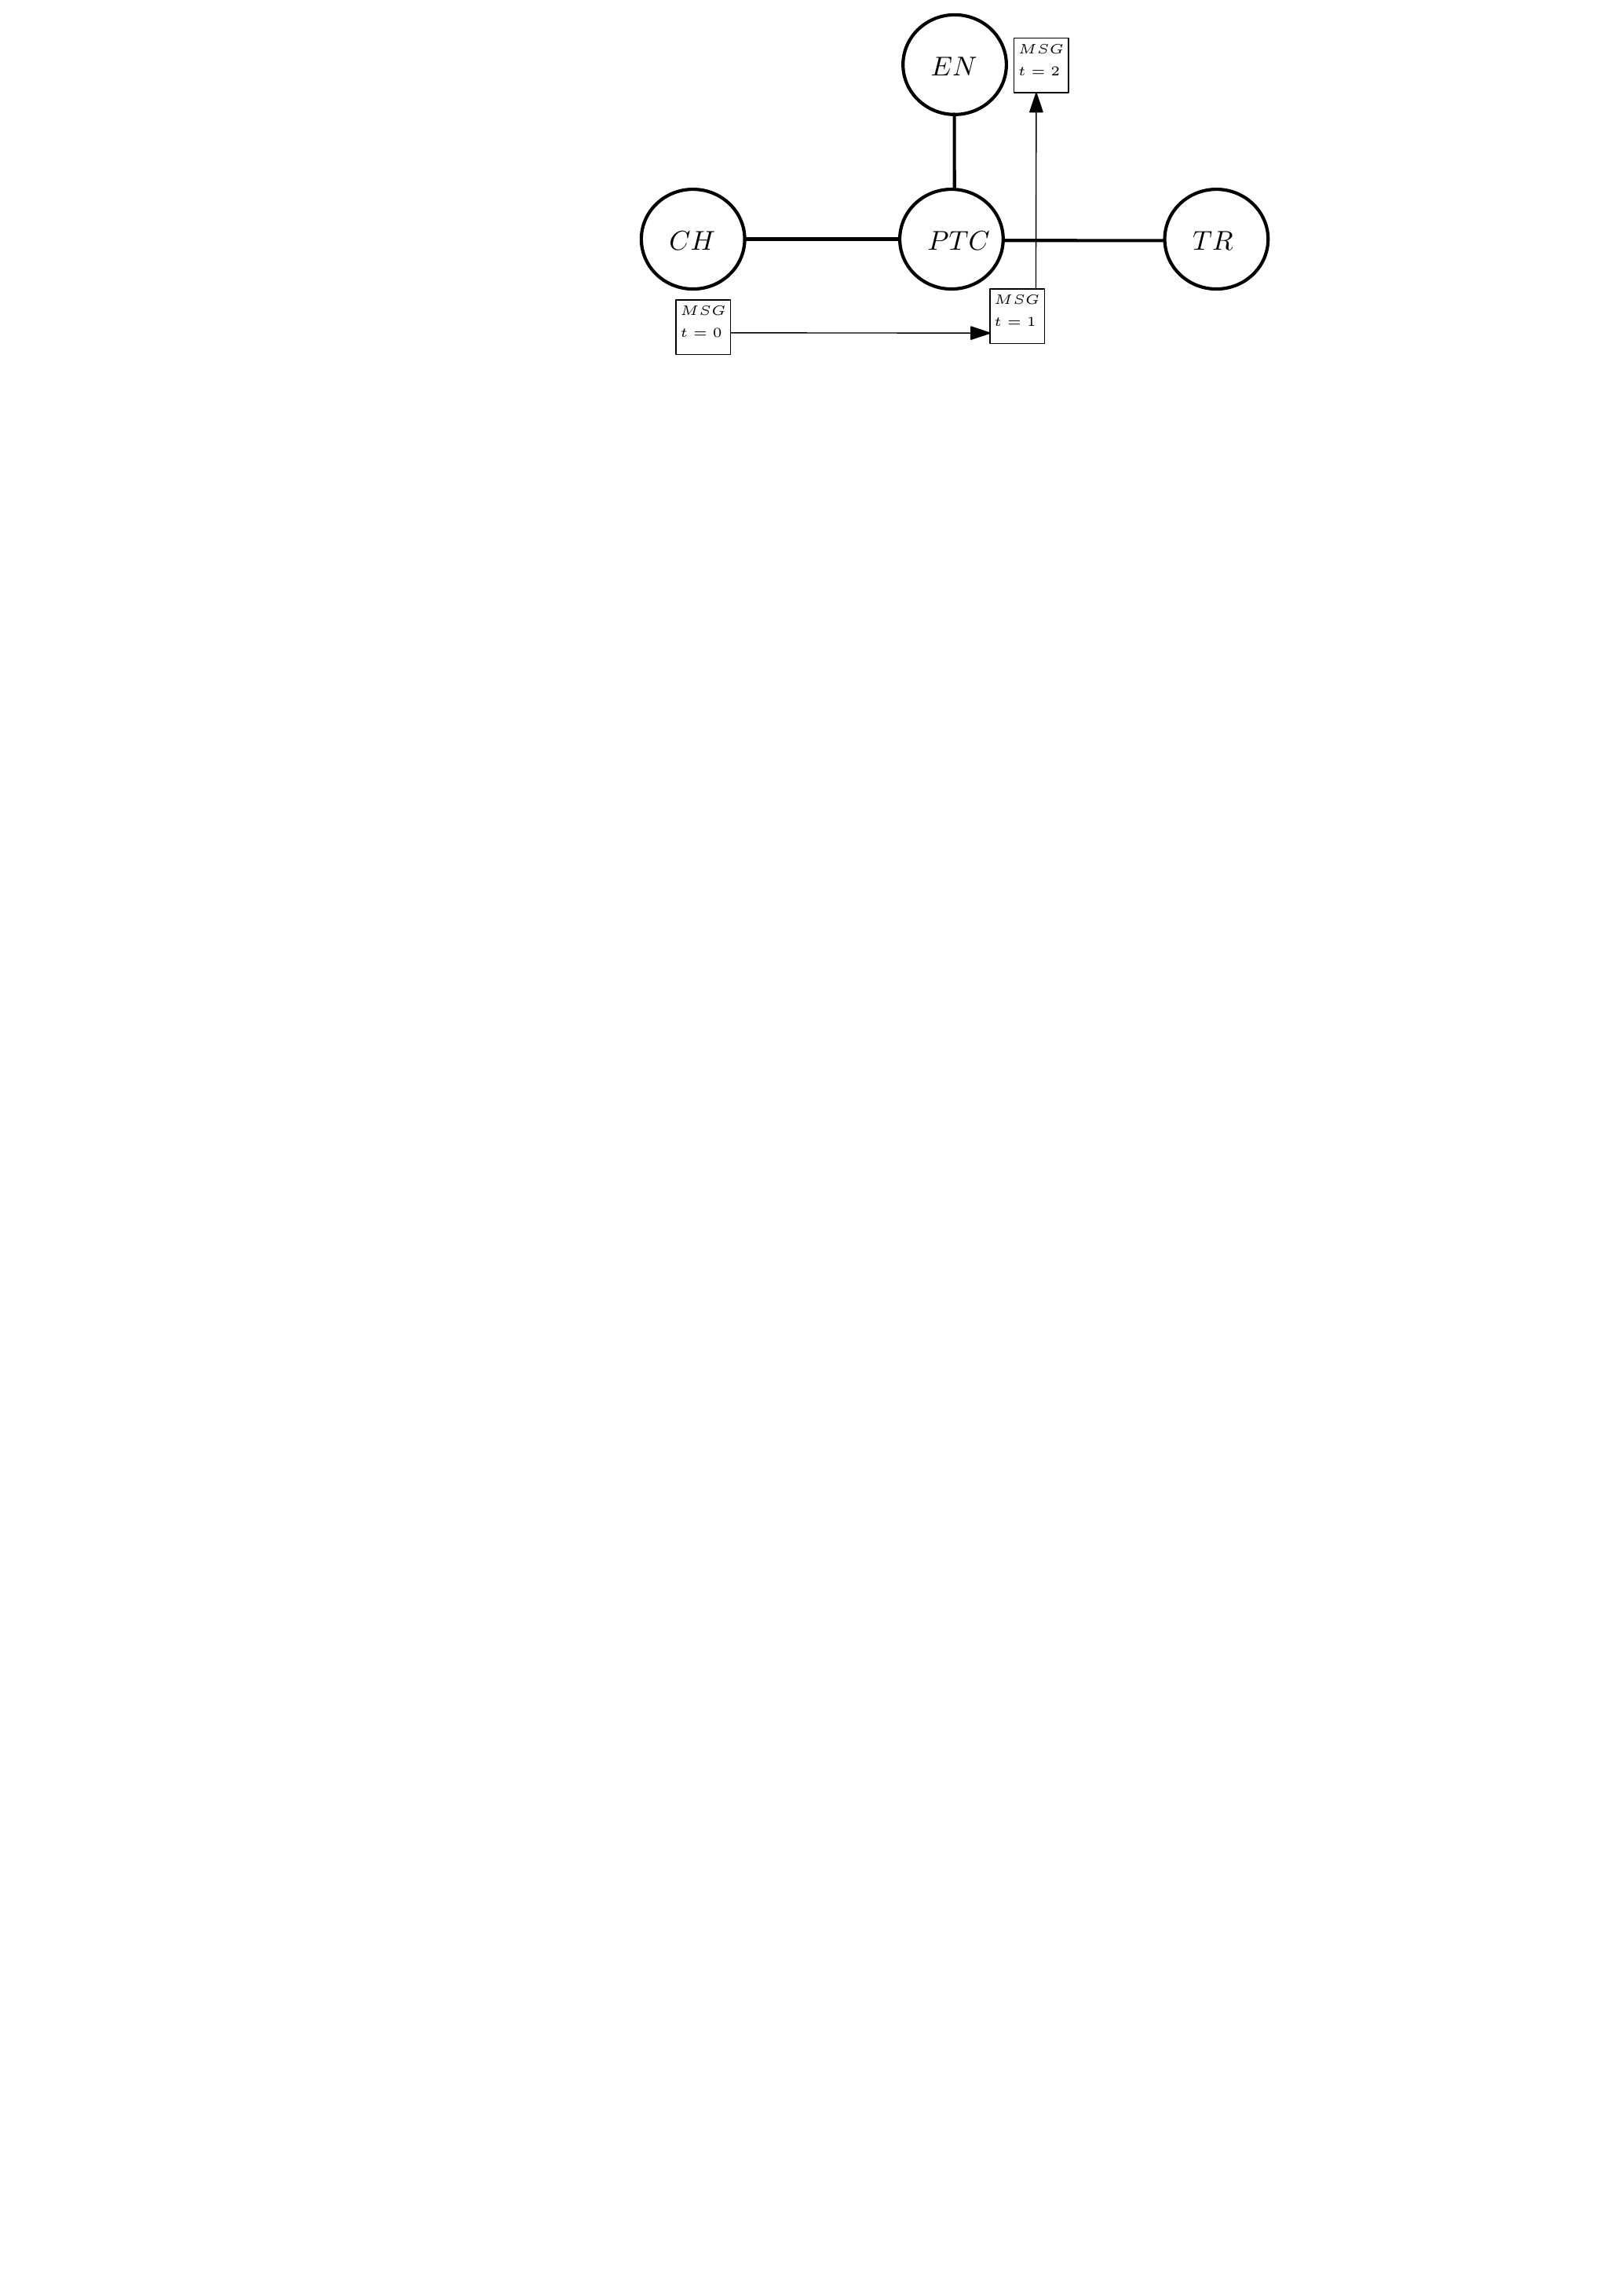}
  \caption{Autosar example message sending}
  \label{fig:RE_msgs}
\end{figure}
\end{example}

\begin{example}
  \label{ex:msgs2}
  In this example we describe the message passing of Request messages
  (in red) and Response messages (in green) in
  Fig.~\ref{fig:msgs-needed}.
  The need of an instanced stream value arises from its presence in
  the right side of an expression in U.
  Therefore a needed value is one such that it is needed to simplify
  that expression, whereas one that is not needed does not appear in
  any expression in U.
  Eager streams always send the Response message to those monitors that
  compute streams that may need their values.
  Lazy streams need to be requested in order to be sent, this way only
  when it is actually needed a Request and matching Response will
  traverse the network.
\qed
\begin{figure}[t]
  \begin{tabular}{cc}
    \includegraphics[scale=0.8]{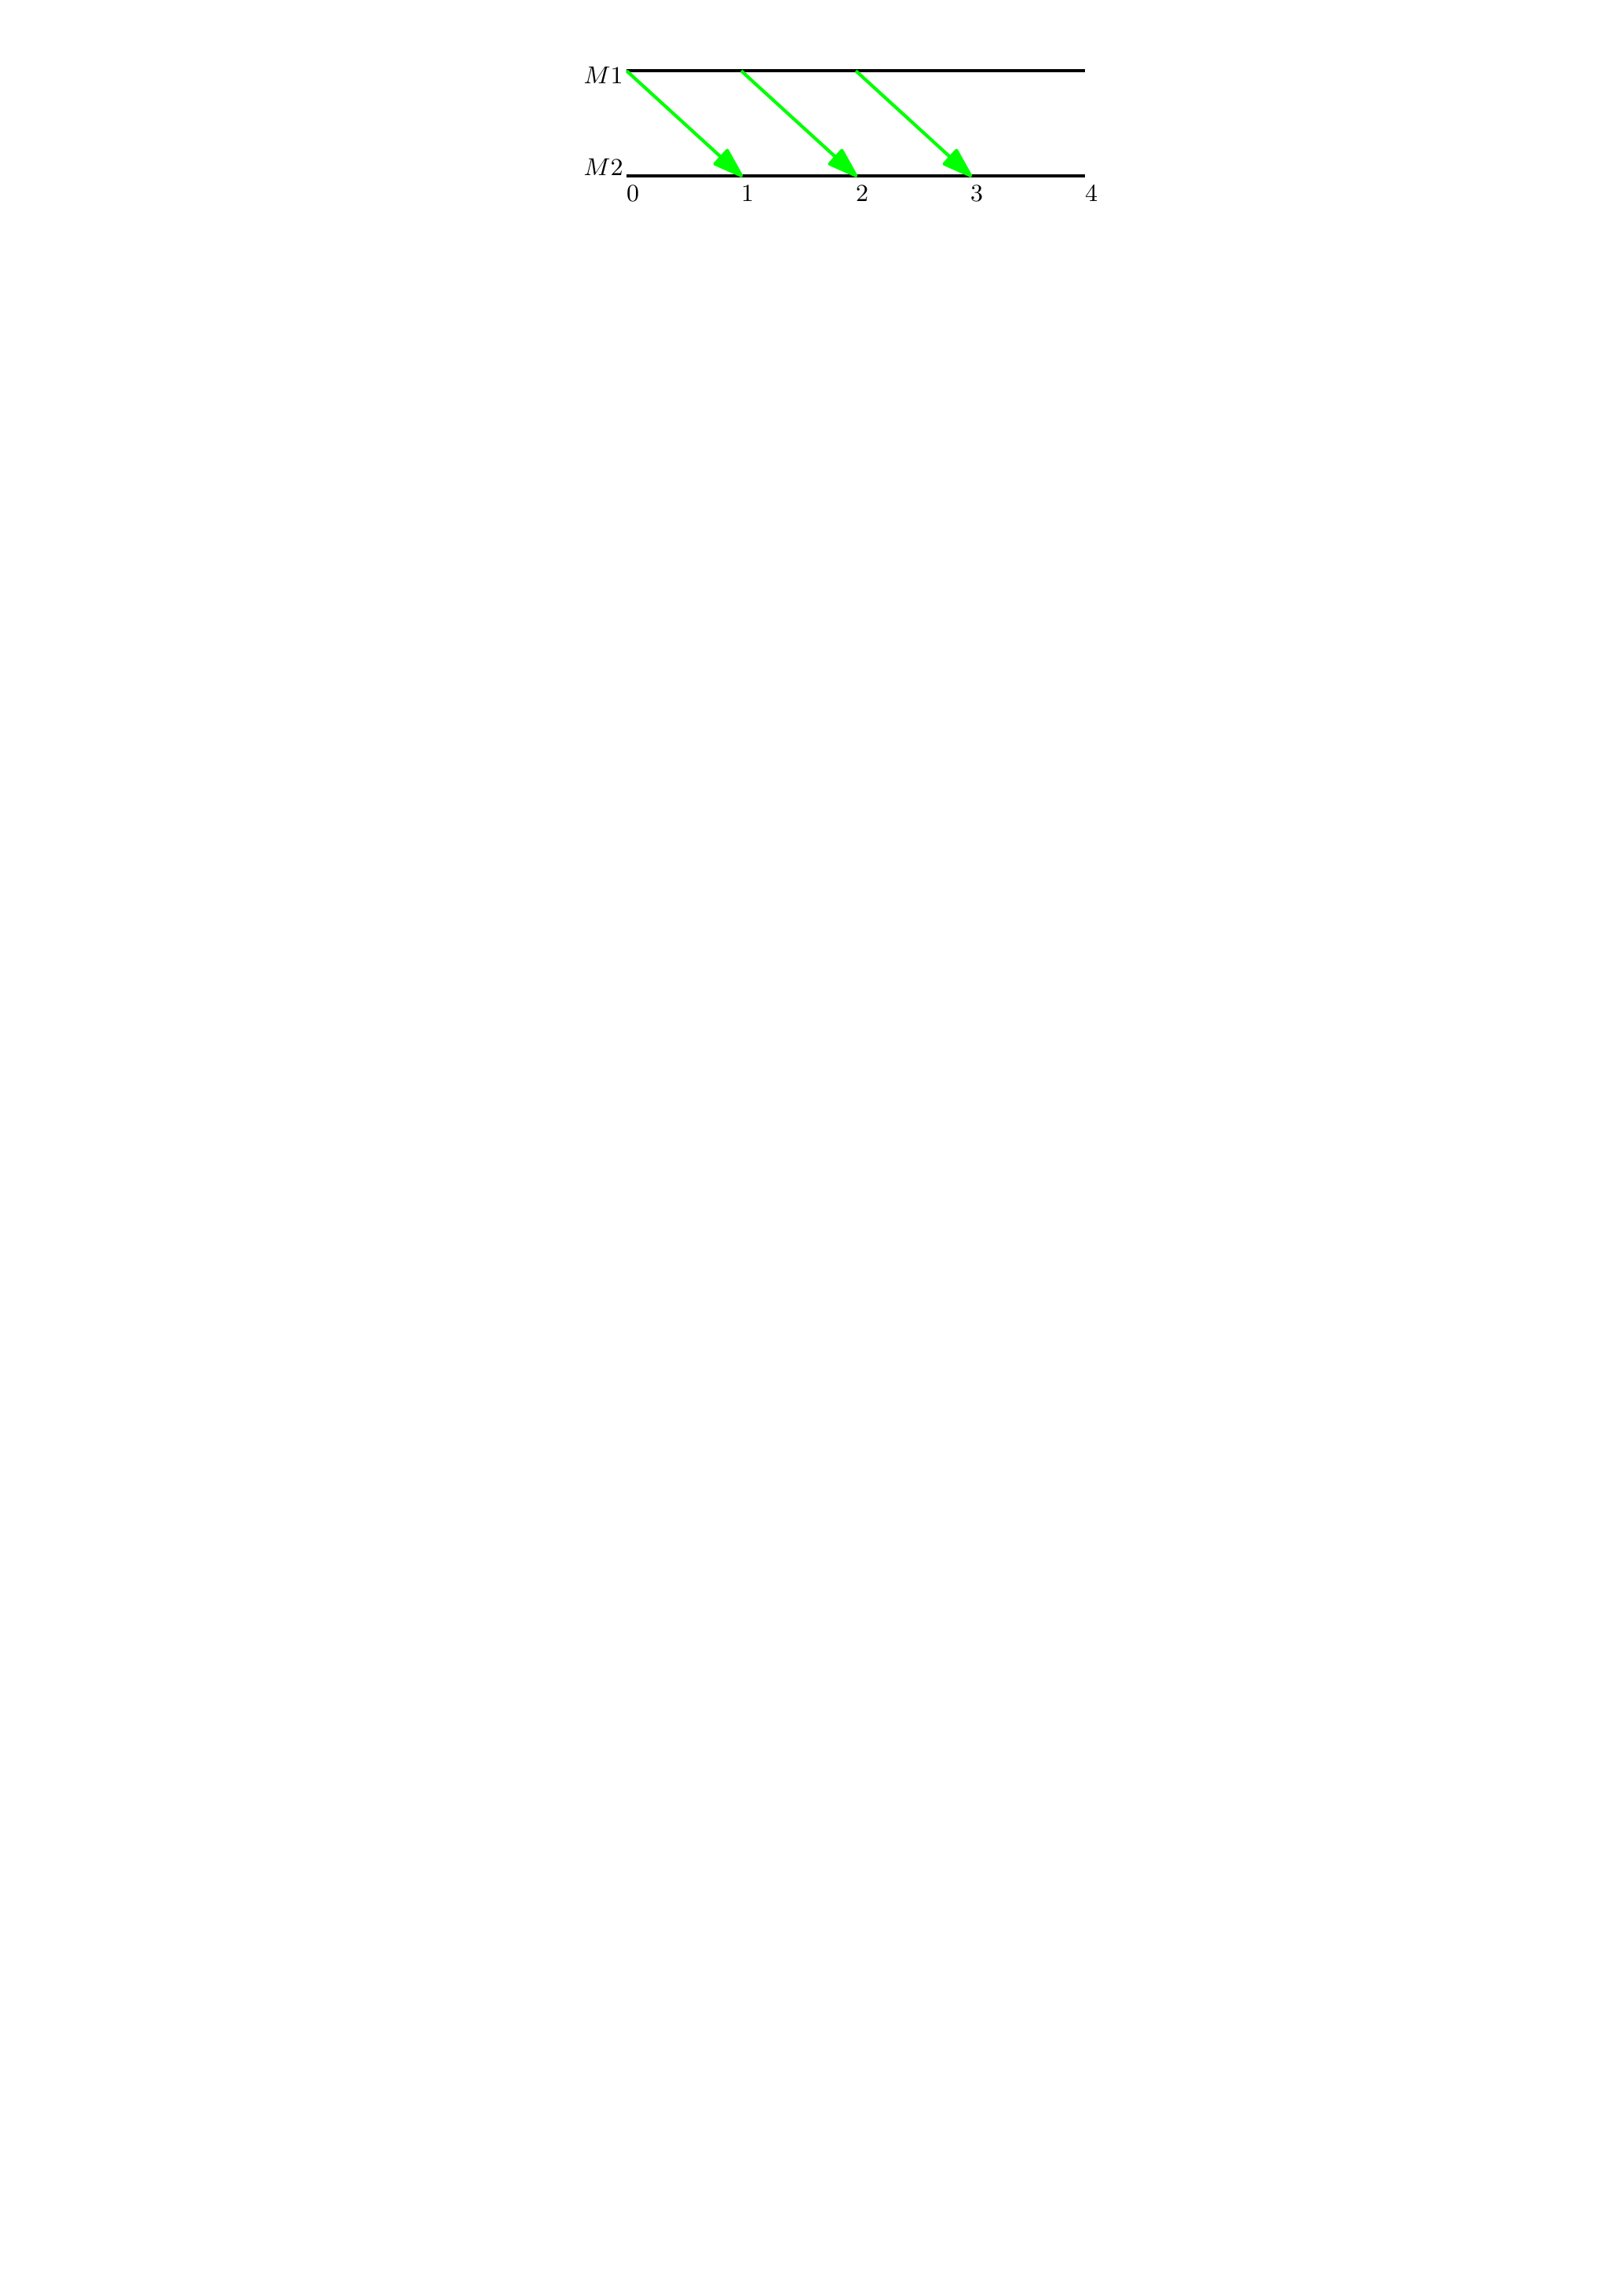} & 
    \includegraphics[scale=0.8]{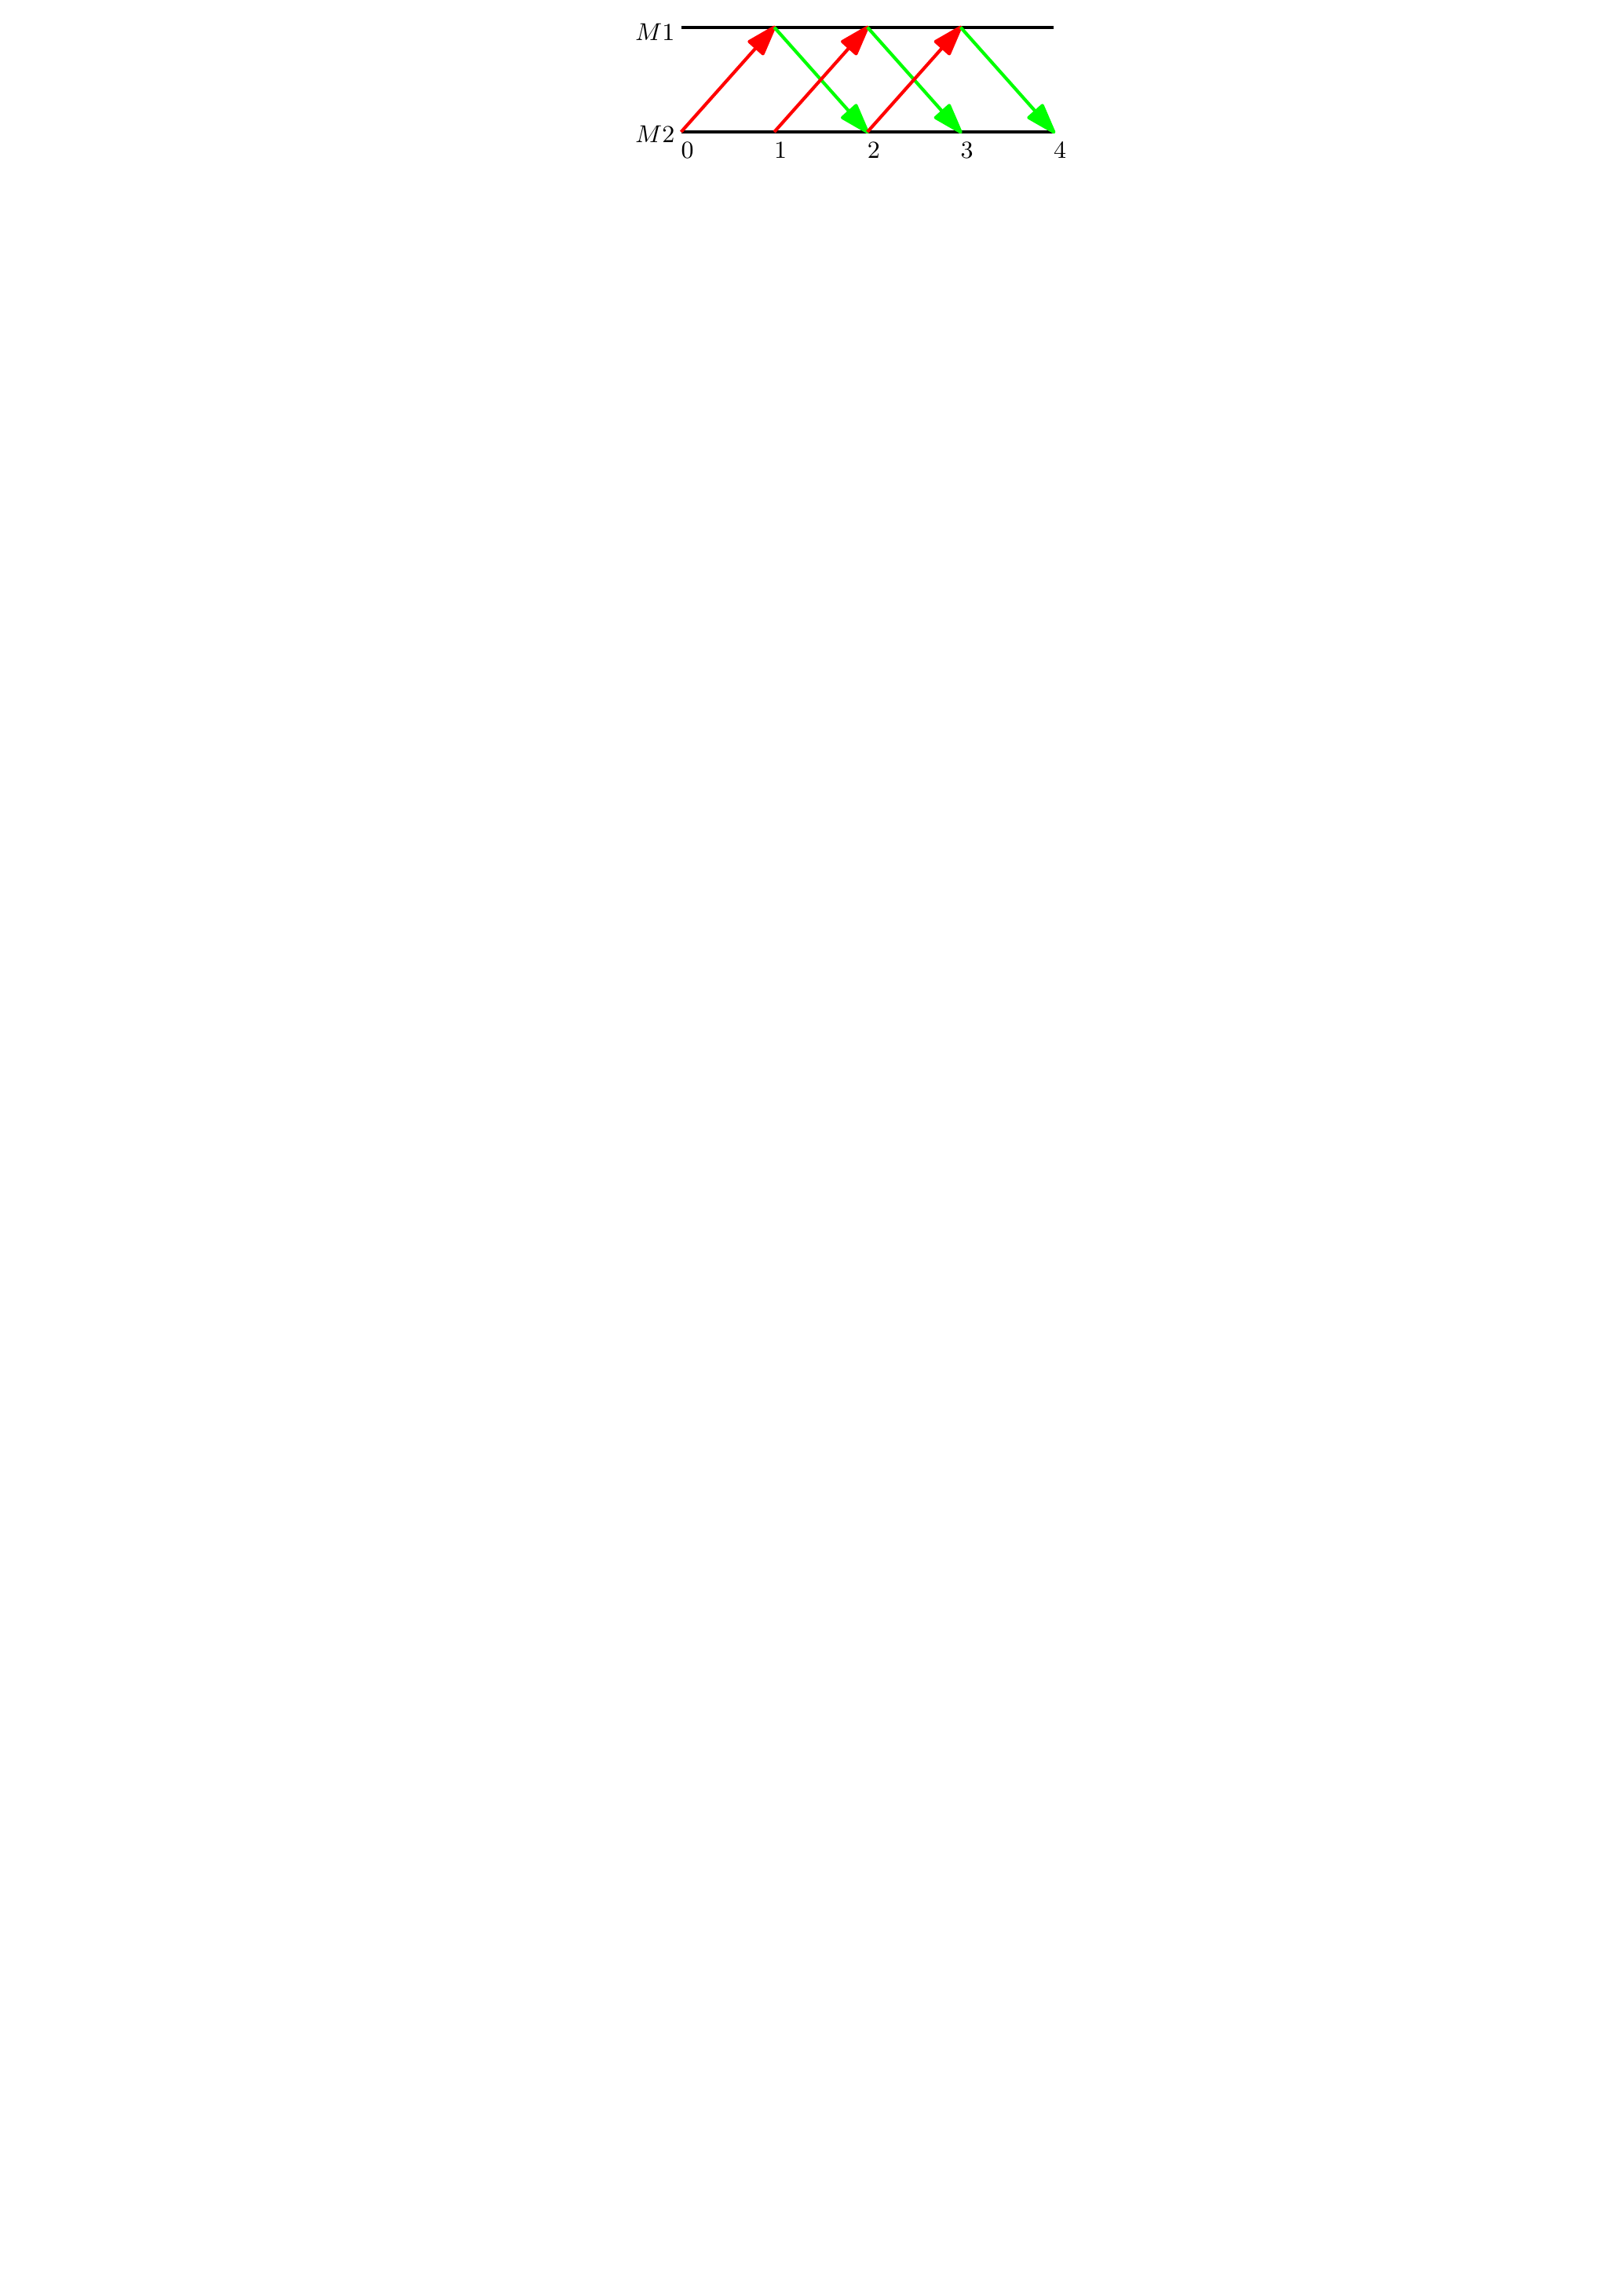}\\
    \text{(a) Eager, all streams are needed} & 
    \text{(b) Lazy, all streams are needed}\\
    \includegraphics[scale=0.8]{RE_eval} & 
    \includegraphics[scale=0.8]{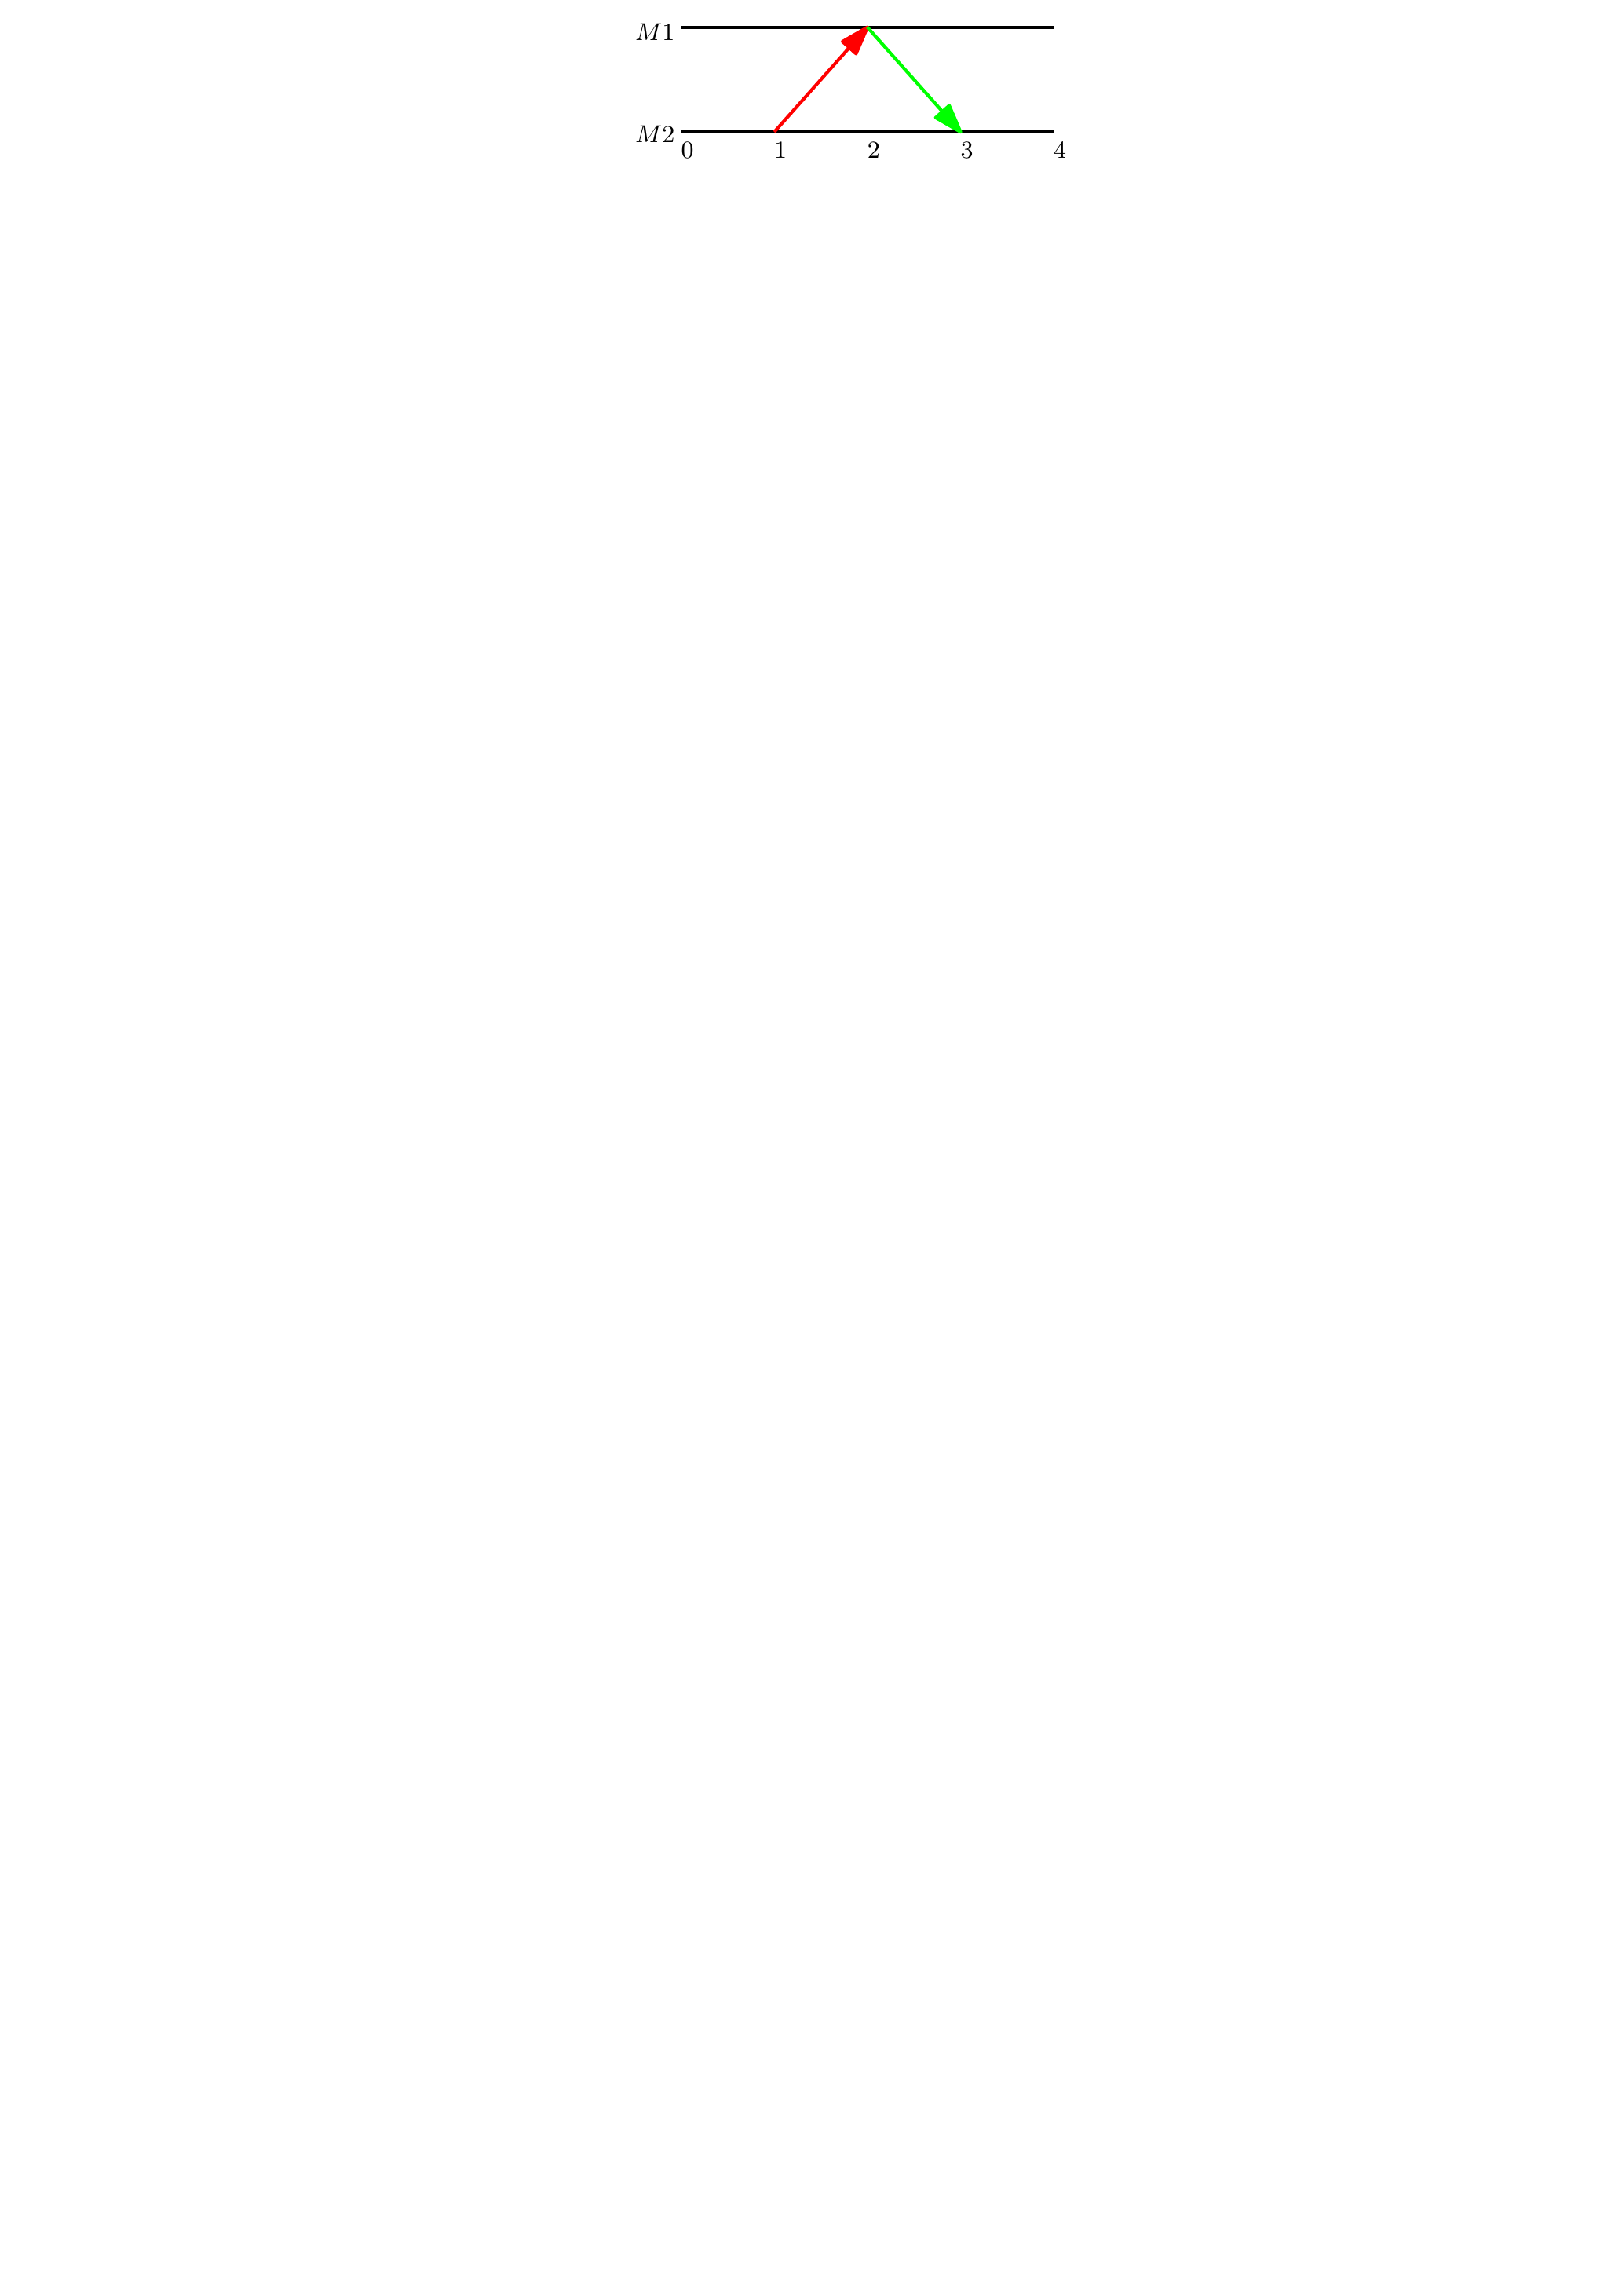}\\
    \text{(c) Eager, rarely the streams are needed} & 
    \text{(d) Lazy, rarely the streams are needed}
  \end{tabular}
  \caption{Messages needed (lazy vs eager)}
  \label{fig:msgs-needed}
\end{figure}
\end{example}

\begin{example}
  \label{ex:full-autosar}
  In this example we propose our solution to the problem of decentralized stream runtime verification in a car that uses the Autosar standard over the CAN network.
  This example is inspired by the Electronic Stability Program (ESP) and models the under steering to the left scenario in an attempt to avoid an obstacle.
  In such a case the ESP must detect the sudden turn of the steering wheel and the deviation produced with the actual movement of the car (yaw).
  When this deviation is perceived and maintained over a period of time, the ESP must act on the brakes, the torque distribution and the engine in order produce the desired movement without any lose of control over the vehicle.
  We define the following streams:
  \begin{compactitem}
  \item $dir\_dev$ which represents the direction of the deviation between the yaw and the steering
  \item $u\_st\_l$ represents the detection of an under steering to the left
  \item $c\_u\_st\_l$ represent the duration of the under steering as a count.
  \end{compactitem}
  {\small\begin{lstlisting}[language=LOLA]
 
clique
@Chassis{
const num dir_tol = 0.2
input num yaw //real wheel direction 100, 100 in percentage
input num steering //driver desired direction 100, 100
input bool drive_wheel_slip 
input num b1 //brakes front left
input num b2 //brakes front right
input num b3 //brake rear left
input num b4 //brakes rear right
const num persistent_threshold = 25
define num dir_dev = steering - yaw //this way we know the direction of the dev

//steering left but car is not moving enough to the left, to avoid an obstacle
define bool u_st_l = dir_dev > 0 and dir_dev > dir_tol 
define num count_u_st_l = if u_st_l then count_u_st_l[-1|0] + 1 else 0
define bool persistent_u_st_l = count_u_st_l > persistent_threshold
define num effective_brake_l_rear = if persistent_u_st_l then count_u_st_l else 0

//other cases: under steering right, and over steering to both sides
output bool ESP_on = u_st_l or drive_wheel_slip //or other cases
//act on throttle
output num req_throttle = if ESP_on then req_throttle[-1|0] - dir_dev else 0
//act on torque distribution
output num req_torque_d = if ESP_on then req_torque_d[-1|0] - dir_dev else 0 
}

@Engine{
input num throttle 
const num throttle_tol = 0.1
output bool correct_throttle = req_throttle[-1|0]/throttle <= throttle_tol
}

@Transmission{
input num torque_d 
const num torque_d_tol = 0.1
output bool correct_torque_d = req_torque_d[-1|0]/torque_d <= torque_d_tol
}

@PowerTrainCoordinator{
output bool all_correct = correct_throttle and correct_torque_d
output bool always_correct = all_correct and always_correct[-1|true]
}

  \end{lstlisting}}

\qed

\end{example}

\clearpage
\section{Efficiently vs Decentralized Efficiently Monitorability}
\label{sec:app:eff-vs-deceff}

Not every efficiently monitorable specification can be evaluated 
with finite memory in the length of the trace.
We show now a counter-example of a efficient monitorable specification
that illustrates that Algorithm~\ref{alg:local-algo} does not run in
bounded memory.
This specification is efficiently monitorable but not decentralized
efficiently monitorable.

Consider the following efficiently monitorable specification deployed
in monitors 1 and 2 with $dist(1,2) = dist(2,1) = 2$:
{\small\begin{lstlisting}[language=LOLA] 
    @1{output num a eval = b[-1|0]} 
    @2{output num b eval = a[-1|0]}
\end{lstlisting}}
It is easy to observe that $a[0]$ and $b[0]$ will be resolved at $t =
0$.  Then, $a[1]$ and $b[1]$ will be resolved at $t = 2$ $a[2]$ and
$b[2]$ will be resolved at $t = 4$ $a[3]$ and $b[3]$ will be resolved
at $t = 6$ so $a[n]$ and $b[n]$ will be resolved at $t = 2n$ which is
not a constant but depends on the time of instantiation and thus it is
unbounded.

% Therefore we can elaborate a claim upon which the decentralized
% algorithm is actually Bounded Memory.
% \begin{theorem}
%   If the Network Deployment Graph is a DAG and the Dependency Graph of
%   the specification is Efficiently Monitorable, then the decentralized
%   algorithm is Bounded Memory.
% \end{theorem}
% In order to prove this we need to prove that every element in U (pair instanced stream, expression) gets resolved $\tUresolved$ in a constant amount of time.
% In order to do that we need a definition
% \begin{definition}
%   Given a specification and its $\delta$ which maps the streams to monitors, then we define $\nabla$ as the time at which a stream gets resolved. $\nabla$ tell us the time needed from a stream is instanced until it is resolved, effectively, the time the pair $(s[t],e) \in U$.
%   Formally, $\nabla(s) = max(0, max(max(0,w_{s,d} + \nabla(d) + dist(\delta(d), \delta(s)))))$ for all $d \in dependencies(s)$.
%   It is always non-negative and is defined by the sum of the future dependencies' shifts plus the nabla of those dependencies plus the distance between the monitors that compute the stream and its dependency.
% \end{definition}
% \begin{proof}
%   .
%   \qed
% \end{proof}
% %END already in efficient

\begin{example}
  \label{ex:decent-efficient}
  In this experiment (see Fig.~\ref{plot:constant-mem}) we can observe
  the bounded memory usage of the specifications independent of the
  trace length, as described in Section \ref{sec:efficient}.
  What we can observe is the average among the maximum memory used for
  the combination of communication strategy (eager, lazy) and mapping
  of stream variables to nodes (centralized, decentralized).
\begin{figure}[tbh!]
  \label{plot:constant-mem}
  \centering
  \includegraphics{plots/constant_memory-crop} 
  \caption{Memory usage}
\end{figure}
\end{example}

\clearpage

\clearpage
\section{Missing proofs}
\label{sec:app:missing}

\newcounter{backup}

\setcounter{backup}{\value{theorem}}
\setcounter{theorem}{\value{thm-convergence}}

\begin{theorem}
  All of the following hold for every instant variable $u[k]$:
  \begin{compactenum}
  \item[\textup{(1)}] If $\ISLAZY(u)$ then all request messages for $u[k]$
    are eventually responded.
    \item[\textup{(2)}] If $\ISEAGER(u)$ then a response message for
      $u[k]$ is eventually sent.
    \item[\textup{(3)}] The value of $u[k]$ is eventually resolved.
    \item[\textup{(4)}] The value of $u[k]$ is $c$ if and only if $(u[k],c)\in R$ at
      some instant.
  \end{compactenum}
\end{theorem}

\setcounter{theorem}{\value{backup}}

\begin{proof}
  Let $M$ be a length of a computation and $\sigma_I$ be an input of
  length $M$.
  Note that $(1)$ to $(4)$ above are all statements about instant
  variables $u[k]$, which are the nodes of the evaluation graph
  $G_{\varphi,M}$.
  We proceed by induction on $G_{\varphi,M}$ (which is acyclic because
  $D_\varphi$ is well-formed).
  \begin{itemize}
  \item \textbf{Base case}: The base case are vertices of the
    evaluation graph that have no outgoing edges, which are either
    instant variables that correspond to inputs or to defined
    variables whose instant equation does not contain other instant
    variables.
    Statement $(3)$ follows immediately for inputs because at instant
    $k$, $s[k]$ is read at node $\mu(k)$.
    For output equations that do not have variables, or whose
    variables have offsets that once instantiated become negative or
    greater than $M$, the value of its leafs is determined either
    immediately or at $M$ when the offset if calculated.
    At this point, the value computed is inserted in $R$, so $(4)$
    also holds at $\mu(u)$.
    Note that $(4)$ also holds for other nodes because the response
    message contains $u[k]=c$ if and only if $(u[k],c)\in R_n$, where
    $\mu(u)=n$.
    If $s$ is eager, then the response message is inserted exactly at
    the point it is resolved, so $(3)$ implies $(2)$.
    Finally, $(1)$ also holds at the time of receiving the request
    message or resolving $u[k]$ (whatever happens later).
  \item \textbf{Inductive case}: Consider an arbitrary $u[k]$ in the
    evaluation graph $G_{\varphi,M}$ and let
    $u_1[k_1],\ldots,u_l[k_l]$ the instant variables that $u[k]$
    depends on.
    These are nodes in $G_{\varphi,M}$ that are lower than $u[k]$ so
    the inductive hypothesis applies, and $(1)$-$(4)$ hold for these.
    Let $n=\mu(u)$.
    At instant $k$, $u[k]$ is instantiated and inserted in $U_n$. 
    At the end of cycle $k$, lazy variables among $u_1[l_1]\ldots
    u_l[ul]$ are requested.
    By induction hypothesis, at some instant all these requests are
    responded by $(1)$.
    Similarly, the values of all eager variables are calculated and
    sent as well (by $(2)$ and $(3)$).
    At the latest time of arrival, the equation for $u[k]$ has no more
    variables and it is evaluated to a value, so $(3)$ holds and $(4)$
    holds at $n$.
    At this point, if $\ISEAGER(u)$ then the response message is sent
    (so $(2)$ holds for $u[k]$) and if $\ISLAZY(u)$ then all requests
    (previously received in $\PEN_n$ or future requests) are answered,
    so $(1)$ also holds.
  \end{itemize}
  This finishes the proof.
  \qed
\end{proof}

\setcounter{backup}{\value{theorem}}
\setcounter{theorem}{\value{thm-correctness}}

\begin{theorem}
  %\label{thm:correctness}
  Let $\varphi$ be a specification, $S:\tupleof{\varphi,\topo,\mu}$ be
  a decentralized SRV problem, and $\sigma_I$ an input.
  Then $(\sigma_I,\OUTPUT(\sigma_I))\models \varphi$.
\end{theorem}

\setcounter{theorem}{\value{backup}}

\begin{proof}
  Let $\sigma_O$ be the unique evaluation model such that
  $(\sigma_I,\sigma_O)\models \varphi$ (we use $\sigma_O(s)$ for the
  output stream for stream variable $s$ and $\sigma_O(s)(k)$ for its
  value in the $k$-th position).  
  We need to show that for every $s$ and $k$,
  $\Osem{s}(k)=\sigma_O(s)(k)$.
  We again proceed by induction on the evaluation graph $G_{\varphi,M}$.
  \begin{itemize}
  \item \textbf{Base case:}
    For inputs the value follows immediately. 
    The other basic case corresponds to output variables $s$ at
    instants at which these that do not depend on other variables
    (because all occurrences of offsets, if any, fall off the trace).
    The evaluation of the value is performed by $\mu(s)$, and it
    satisfies the equation $e_s$ of $s$, not depending on any value of
    any other stream. 
    Therefore, it satisfies that $\Osem{s}(k)=\sem{e_s[k]}=\sigma_O(s)(k)$,
    as desired
  \item \textbf{Inductive case:} 
    Let $s$ be an arbitrary stream variable and $k$ an arbitrary
    instant within $0$ and $M-1$ and assume that all instant variables
    $u[k']$ that $s[k]$ can reach in the evaluation graph satisfy the
    inductive hypothesis.
    Let $n$ be the node in charge of computing $s$.
    By Theorem~\ref{thm:convergence}, all the values are eventually
    received by $n$ and in $R_n$, and by IH, these values are the same
    as in the denotational semantics, that is
    $\Osem{u}(k')=\sigma_O(u)(k')$.
    The evaluation of $s[k]$ corresponds to computing $\sem{e_s}$,
    which uses the semantics of the expression (according to
    Section~\ref{sec:lola}).
    A simple structural induction on the expression $e_s$ shows that
    the result of the evaluation, that is the value assigned to
    $s[k]$, is $\sem{e_s}_{\sigma}(k)=\sigma_O(s)(k)$, as desired.
  \end{itemize}
  This finishes the proof.
  \qed
\end{proof}
